# Supplementary material for: Non-contact Lung Disease Classification via OFDM-based Passive 6G ISAC Sensing
Source: arXiv:2405.09458 source file (2024-05-15)
Supplement: Supplementary file 1 [file appendix.tex]

\section{Computation of $\mathcal{L}_{I_{J}}(s)$ for IoT transmission on the downlink}
%\label{sec:Appendix}

The Laplace transform of the cumulative interference ${I_J}$ is defined as:

\begin{align}
%{L_{I_{J}}}(s)=E_{I_{J}}exp(-s I_{J}) \\
\mathcal{L}_{I_{J}}(s)=\mathbb{E}_{I_{J}}\biggl[\exp(-s I_{J})\biggl],
\end{align}

\begin{align}
\mathcal{L}_{I_{J}}(s)=\mathbb{E}_{\phi_j,\{|h_j|^2\}}\biggl[\exp\biggl(-s {\sum_{j\in\phi_{J}}{P_{j}}|h_j|^2{\Vert\mathbf{X}_j\Vert^{-\alpha}}}\biggl)\biggl].   
\end{align}

Next, we use the property of the exponential function that the sum of exponential powers is the product of exponentials and  put the value of $s$ back in the above expression to get: 

\begin{align}
\mathcal{L}_{I_{J}}(s)=\mathbb{E}_{\phi_j,\{|h_j|^2\}}\biggl[\prod_{{j\in\phi_{J}}}exp\biggl(- |h_j|^2\biggl(\dfrac{P_{j}}{P}\biggl) {\beta_D } {\Vert\mathbf{X}_j\Vert^{-\alpha}}{r^{\alpha}}\biggl)\biggl].
\end{align}
Let $\gamma_{j} ={P_{j}}/{P}$, as $\phi_j$ is independent with $|h_j|^2$ we can take one expectation (i.e., $\mathbb{E}_{\{|h_j|^2\}}$) inside, which is given below:

\begin{align}
\label{eq:PGFL}
\mathcal{L}_{I_{J}}(s)=\mathbb{E}_{\phi_j}[\prod_{{j\in\phi_{J}}}\mathbb{E}_{\{|h_j|^2\}}[exp(- |h_j|^2\gamma_{j} {\beta_D } (\dfrac{\Vert\mathbf{X}_j\Vert}{r})^{-\alpha})]].
\end{align}
%\begin{align}
%=\mathbb{E}_{\phi_j}\biggl[\prod_{{j\in\phi_{J}}}\dfrac{1}{1+{\gamma_{j} {\beta_D } \biggl(\dfrac{\Vert\mathbf{X}_j\Vert}{r}\biggl)^{-\alpha}}}\biggl] \nonumber
%\end{align}

Indeed, Eq. \ref{eq:PGFL} is the Probability Generating FunctionaL (PGFL) of PPP, which can be expressed as:

\begin{align}
&\mathcal{L}_{I_{J}}(s)= \\& \exp\biggl(-\rho_J \bigintsss_{\mathcal{A}}1-\mathbb{E}_{|h|^2}[exp(- |h|^2\gamma_{j} {\beta_D } (\dfrac{\Vert\mathbf{x}\Vert}{r})^{-\alpha})] d\mathbf{x}\biggl), \nonumber
\end{align}
where $\rho_J$ is the intensity of jammer nodes, $\mathcal{A}$ is the effective 2D area where jammers signals are prominent or can affect the transmissions.
Now, converting $x$ into polar form as $x=(r_j, \theta)$ ($j$ subscript is used in order to differentiate it from the earlier used $r$ (distance of follower)), we have,
\begin{align}
&\mathcal{L}_{I_{J}}(s)= \\& \exp\biggl(-2\pi\rho_J \bigintsss_{z_1}^{z_2}\biggl(1-\mathbb{E}_{|h|^2}[exp(- |h|^2\gamma_{j} {\beta_D } (\dfrac{{r_j}}{r})^{-\alpha})]\biggl) r_j dr_j\biggl), \nonumber
\end{align}
 which can be written as:
%\gamma_{j} {\beta_D } (\dfrac{{r_j}}{r})^{-\alpha}

\begin{align}
\mathcal{L}_{I_{J}}(s)=\exp\biggl(-2\pi\rho_J \bigintsss_{z_1}^{z_2}\biggl(1-\dfrac{1}{1+ \biggl(\gamma_{j} {\beta_D } (\dfrac{{r_j}}{r})^{-\alpha}\biggl)^{}}\biggl) r_{j} dr_j\biggl),
\end{align}
which can be further simplified as

\begin{align}
\mathcal{L}_{I_{J}}(s)=\exp\biggl(-2\pi\rho_J \bigintsss_{z_1}^{z_2}\biggl(\dfrac{1}{1+ \biggl((\gamma_{j} {\beta_D })^{-1} (\dfrac{{r_j}}{r})^{\alpha}\biggl)^{}}\biggl) r_{j} dr_j\biggl),
\end{align}
where $z_1$ and $z_2$ constitute
the effective attacking area of the jammers, s.t., $z_1 < z_2$, or the area from where jammers can significantly affect the transmissions.
 To make the expression elegant let $u=\biggl({r_{j}}/{r({\gamma_{j} {\beta_D })^{{1}/{\alpha}}}}\biggl)^{2} $, $z_l=\biggl(\dfrac{z_1}{r(\gamma_{j} \beta_D )^{{1}/{\alpha}}}\biggl)^2$ and $z_u=\biggl(\dfrac{z_2}{r(\gamma_{j} \beta_D )^{1/\alpha}}\biggl)^2$,
 then the above expression can be written as:
\begin{align}
\mathcal{L}_{I_{J}}(s)=\exp\biggl({-\pi\rho_J }{r^2 (\gamma_{j} \beta_D )^{{2}/{\alpha}} } \bigintsss_{z_l}^{z_u}\dfrac{1}{1+(u^{\alpha/2})}du\biggl).
\end{align}
Integral is computed via Gauss-hypergeometric approximation, given as:
\begin{equation}
\begin{split}
& \mathcal{L}_{I_{J}}(s)= \\
   & \exp\biggl(\dfrac{\pi \rho_J \gamma_{j}\beta_D r^{\alpha}}{(\alpha/2)-1} \biggl( z_2^{(2-\alpha)}{}_{2}F_{1}(1,1-{\dfrac{2}{\alpha}},2-{\dfrac{2}{\alpha}},-\gamma_j \beta_D (\dfrac{r}{z_2})^\alpha)\\
&    - z_1^{(2-\alpha)} {}_{2}F_{1}(1,1-{\dfrac{2}{\alpha}},2-{\dfrac{2}{\alpha}},-\gamma_j \beta_D (\dfrac{r}{z_1})^\alpha) \biggl)\biggl).
\end{split}
\end{equation}

%%%%%%%%%%%%%%%%%%%%%%%%%%%%%%%%%%%%%%%%%%%%%%%%
%%%%%%%%%%%%%%%%%%%%%%%%%%%%%%%%%%%%%%%%%%%%%%%%
%%%%%%%%%%%%%%%%%%%%%%%%%%%%%%%%%%%%%%%%%%%%%%%%%%%
